# Supplementary material for: Pressure-Tunable Targets for Light Dark Matter Direct Detection: The Case of Solid Helium
Source: arXiv:2409.02439 source file (2024-09-04)
Supplement: Supplementary file 1 [file supplemental_material.pdf]

# Supplemental Material for
# Pressure-Tunable Targets for Light Dark Matter Direct Detection: The Case of Solid Helium

Omar A. Ashour[1, 2, 3] and Sinéad M. Griffin[2, 3, *]

[1] *Department of Physics, University of California, Berkeley, California 94720, USA*
[2] *Materials Sciences Division, Lawrence Berkeley National Laboratory, Berkeley, CA 94720, USA*
[3] *Molecular Foundry, Lawrence Berkeley National Laboratory, Berkeley, CA, 94720, USA*

(Dated: September 4, 2024)

## COMPUTATIONAL METHODS

All Density Functional Theory (DFT) calculations, except for the hybrid and meta-GGA functionals, use Quantum ESPRESSO 7.2 [1, 2] along with the projector augmented wave (PAW) [3] dataset from `pslibrary` v1.0.0 [4]. All the calculations in the main text use the PBE functional [5], combined with the D3M dispersion correction [6, 7]. We set the wavefunction energy cutoff at 120 Ry and the charge density energy cutoff at 960 Ry. The electronic structure calculations for the $\alpha$ and $\beta$ phases were performed using $\Gamma$-centered $k$-point grids of $20\times20\times12$ and $20\times20\times20$, respectively. Constrained relaxations were performed, maintaining the cell shape and Bravais lattice while targeting specific pressures. The pressure was converged to within, at most, 0.05 GPa. For hybrid and meta-GGA functionals, we used VASP 6.4.1 [8–12] with the `potpaw.54` PAW dataset. We found it imperative to use the `He_GW` PAW dataset with VASP due to inconsistencies with the standard `He POTCAR` when comparing results to those from Quantum ESPRESSO using multiple pseudopotentials.

Phonons were calculated using density functional perturbation theory (DFPT), as implemented in Quantum ESPRESSO, or the finite differences approach using VASP in conjunction with `phonopy` [13]. We used a $3\times3\times3$ $q$-grid, or a supercell of the same dimensions, converging phonons energies to within $\mathcal{O}(10\,\mu\text{eV})$ of a $4\times4\times4$ $q$-grid. The average phonon frequencies across the entire Brillouin zone (BZ), $\langle\omega\rangle$, were computed using a $20\times20\times20$ $q$-grid using `phonopy`. The average longitudinal optical phonon frequency near the $\Gamma$ point, $\langle\omega_{\text{LO}}(\Gamma)\rangle$, and the average speed of sound, $\bar{c}_S^{LA}$, were calculated by averaging over the surface of a sphere with radius $q = 10$ eV, centered at the $\Gamma$ point.

We performed the DM scattering rate, projected reach, and daily modulation calculations using our package `DarkMAGIC v0.0.4` [14], which implements the effective field theory of Refs. [15, 16], and will be detailed in a forthcoming publication. We used a spherical grid with dimensions $80\times40\times40$ ($n_r\times n_\phi\times n_\theta$) to sample the DM momentum transfer, and a $30\times30\times30$ Monkhorst-Pack grid, shifted from the $\Gamma$ point by half a step, to sample the first BZ when computing the Debye-Waller factor (Eq. (5) in the main text).

## REFERENCE CROSS SECTION

The reference cross section $\bar{\sigma}_n$ for the hadrophilic scalar mediator model is given by

$$\bar{\sigma}_n \equiv \frac{\mu_{\chi n}^2}{\pi}\overline{|\mathcal{M}_{\chi n}(q=q_0)|} = \frac{\mu_{\chi n}^2}{4\pi}\frac{y_\chi^2 f_n^2}{\left(m_\chi^2 v_0^2 + m_\phi^2\right)^2}$$
$$= \frac{\mu_{\chi n}^2 y_\chi^2 f_n^2}{4\pi} \times \begin{cases} m_\phi^{-4} & \text{(heavy mediator)} \\ (m_\chi v_0)^{-4} & \text{(light mediator)} \end{cases} \tag{S1}$$

where $\mu_{\chi n}$ is the DM-neutron reduced mass, and $v_0$ is the DM velocity dispersion.

## NUCLEAR FORM FACTOR

A conventional choice [17] for the nuclear form factor is that of Helm [18], which is isotropic and given by

$$F_N(q) = \frac{3J_1(qr_n)}{qr_n}e^{-(qs)^2/2},$$
$$r_n \simeq 1.14A_n^{1/3}\,\text{fm}, \quad s \simeq 0.9\,\text{fm}. \tag{S2}$$

Here, $J_1$ is an order 1 spherical Bessel function of the first kind, $A_n$ is the atomic number, and $q$ is the momentum transfer. $r_n$ and $s$ are the effective nuclear radius and the nuclear skin thickness, respectively. Note that $F_N(q) \to 1$ as $q \to 0$. For a helium nucleus $F_N(q) - 1 \sim 10^{-7}$ for all DM masses (and thus momentum transfers) considered in this work. Our calculations explicitly set $F_N(q) = 1$.

## DARK MATTER VELOCITY DISTRIBUTION

We assume a truncated Maxwell-Boltzmann (MB) distribution boosted by the Earth's velocity with respect to the galactic rest frame [15]

$$f_\chi^{\text{MB}}(\boldsymbol{v}) = \frac{1}{N_0}e^{-(\boldsymbol{v}+\boldsymbol{v}_\text{e})^2/v_0^2}\Theta\left(v_\text{esc} - |\boldsymbol{v}+\boldsymbol{v}_\text{e}|\right) \tag{S3}$$

where

$$N_0 \equiv \pi^{3/2} v_0^2 \left[ v_0 \,\mathrm{erf}\,(v_{\rm esc}/v_0) - \frac{2v_{\rm esc}}{\sqrt{\pi}} \exp\left(-v_{\rm esc}^2/v_0^2\right) \right]. \tag{S4}$$

Here, $v_0 = 220\,\mathrm{km/s}$ is the dispersion of the distribution, which is truncated by $v_{\rm esc} = 500\,\mathrm{km/s}$, the galactic escape velocity, and boosted to the target rest frame by $\boldsymbol{v}_{\rm e}$, the Earth's velocity with respect to the DM wind, with a mean of $v_{\rm e} \approx 240\,\mathrm{km/s}$.

## REACH OF $\beta$-HELIUM

The single-phonon reach of $\beta$-Helium is shown in Fig. S1 for both mediators.

## DAILY MODULATION

We computed the daily modulation using a similar setup to Ref. [20]. We oriented the crystals so that the $c$- and $\langle 111 \rangle$-axes of the $\alpha$ and $\beta$ phases aligned with the DM wind at $t = 0$. In Fig. S2 we plot the rate $R$, normalized by the average daily rate $\langle R \rangle$, for both phases and mediators at several representative pressures. At a given pressure, acoustic phonons have little to no reach in the shaded DM mass region, so we excluded it from our analysis. We then define the total variation in the normalized rate as

$$\Delta R \equiv (\max(R) - \min(R))/\langle R \rangle \tag{S5}$$

and plot it in Fig. S3 as a function of DM mass and pressure.

## PHONONIC PROPERTIES AS A FUNCTION OF PRESSURE

Figure S4 illustrates the relationship between pressure and various phononic properties: the average phonon frequencies $\langle \omega \rangle$, the average longitudinal optical phonon frequency near the $\Gamma$ point, $\langle \omega_{\rm LO}(\Gamma) \rangle$, and the directionally averaged speed of sound, $\bar{c}_S^{LA}$.

As shown in the previous section, the features of the daily modulation are largely unaffected by pressure, except for the notable shift to lower masses. This effect arises because the phononic spectra are qualitatively similar across all pressures examined, and their features remain unchanged beyond an increase in the average phonon frequencies, as shown in Figs. S5 and S6.

TABLE S1: The exchange-correlation (XC) functionals benchmarked for solid helium. GGA denotes the generalized-gradient approximation. Dispersion corrections labeled with (BJ) use Becke-Johnson damping. The nonlocal van der Waals density functional (vdW-DF) functionals were originally introduced in Ref. [24].

| Functional | Type | Reference |
|---|---|---|
| PBE | GGA | [5] |
| PBEsol | GGA | [25] |
| PBE-D3[a] | Dispersion-corrected GGA | [5, 6] |
| PBE-D3(BJ)[a] | Dispersion-corrected GGA | [5, 6, 26] |
| PBE-D3M[a] | Dispersion-corrected GGA | [5–7] |
| PBE-D3M(BJ)[a] | Dispersion-corrected GGA | [5–7] |
| PBE-MBD | Dispersion-corrected GGA | [5, 27] |
| PBE-TS | Dispersion-corrected GGA | [5, 28] |
| PBEsol-D3 | Dispersion-corrected GGA | [6, 25] |
| HSE06 | Hybrid | [29] |
| HSEsol | Hybrid | [30] |
| HSE06-D3 | Dispersion-corrected hybrid | [6, 29] |
| HSE06-D3(BJ) | Dispersion-corrected hybrid | [6, 26, 29] |
| HSEsol-D3 | Dispersion-corrected hybrid | [6, 30] |
| optB86b-vdW | Nonlocal vdW-DF | [31] |
| vdW-DF-C6 | Nonlocal vdW-DF | [32] |
| vdW-DF-cx | Nonlocal vdW-DF | [33] |
| vdW-DF3-opt1 | Nonlocal vdW-DF | [34] |
| vdW-DF3-opt2 | Nonlocal vdW-DF | [34] |
| rVV10 | Nonlocal vdW-DF | [35] |
| SCAN + rVV10 | Meta-GGA + vdW-DF | [35, 36] |
| r2SCAN + rVV10 | Meta-GGA + vdW-DF | [35, 37] |

[a] Tested with and without three-body terms.

## PERFORMANCE OF DIFFERENT XC FUNCTIONALS

To determine the optimal exchange-correlation (XC) functional and dispersion correction for modeling helium at high pressures, we assessed the structural and vibrational properties using a range of semi-local, hybrid, and meta-GGA functionals. These calculations were performed at the two smallest molar volumes for each phase where experimental data was available: 11.61 and 9.41 $\mathrm{cm^3/mol}$ for the $\alpha$ phase and 11.72 and 9.03 $\mathrm{cm^3/mol}$ for the $\beta$ phase. The results were compared against inelastic neutron scattering data at those same volumes, with corresponding experimental pressures of 168 MPa [21] ($\alpha$) and 136 MPa [22] ($\beta$) at the larger volumes, and 410 MPa [21] ($\alpha$) and 493 MPa [23] ($\beta$) at the smaller volumes. We used the experimental lattice constants in these calculations, without relaxation. Table S1 lists all the functionals employed in our analysis.

Our comparison between DFT predictions and experimental data is visually represented in Fig. S7 for low-pressure structures and in Fig. S8 for high-pressure structures. The semi-local functionals, even with the inclusion of dispersion corrections, consistently underestimate

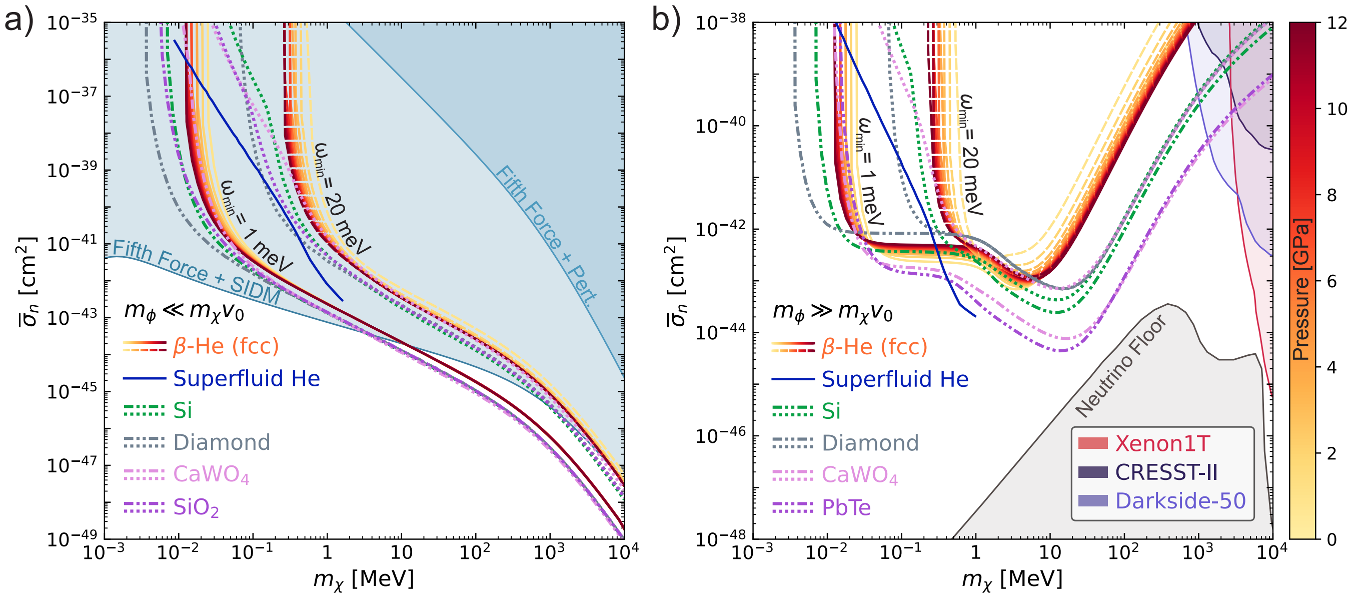


FIG. S1: (a, b) Single-phonon projected reach for light and heavy scalar mediators, respectively. Gradient colored lines correspond to $\beta$-helium under different pressures between 1 (light orange) and 12 GPa (dark red), with solid colors representing other materials. For helium, solid, dashed, and dash-dotted lines correspond to 1 meV, 20 meV, and 100 meV detector thresholds ($\omega_{\rm min}$), while for other materials, dash-double-dotted and dotted lines correspond to $\omega_{\rm min} = 1$ and 20 meV. The solid navy line corresponds to multiphonon scattering in superfluid helium with $\omega_{\rm min} \sim 1$ meV [19]. The constraints are the same as Fig. 3 in the main text.

phonon energies in lower pressure structures, as shown in Fig. S7a and S7c. In contrast, the vdW-DF functionals with nonlocal corrections exhibit better performance, particularly in the $\alpha$ phase, where vdW-DF-C6 closely aligns with experimental observations (see Fig. S7b). However, all functionals we evaluated failed to accurately describe the lower pressure fcc structure, with selected results depicted in Fig. S7d. In our evaluation of the PBE functional augmented with dispersion corrections, we also investigated the impact of incorporating three-body terms, finding negligible differences in the resulting phonon dispersions.

Conversely, higher-pressure structures are accurately represented by dispersion-corrected semi-local functionals, as shown in Fig. S8a and S8c. Notably, uncorrected PBE gives excellent results, exceeding standard D3 corrections, and matches closely with the PBE-D3M configuration selected for the calculations in the main text. In contrast, nonlocal functionals underperform in both high-pressure structures, consistently overestimating phonon energies, which is clearly illustrated in Fig. S8b and S8d.

We also evaluated several of the functionals listed in Table S1 for their ability to reproduce the experimental equation of state [38], with a subset of these results presented in Fig. S9. At lower pressures below 0.5 GPa, the nonlocal van der Waals density functionals (vdW-DF) marginally outperform both the semi-local and dispersion-corrected semi-local functionals. However, at higher pressures, all three classes of functionals give comparable results.

## COMPARISON OF DFT CALCULATION TO EXPERIMENT

Comparing our DFT calculations to inelastic neutron scattering data at ~400-500 MPa [21, 23], we find excellent agreement, as shown in Fig. 2(a,b). Additional testing at ~100 MPa (Fig. S7) shows that DFT fails to model phonons in helium at lower pressures accurately, so we restrict ourselves to higher pressures in this work. Since there is a lack of neutron scattering data at pressures above 500 MPa, we verify our approach against the equation of state (EOS) and the directionally-averaged group velocity of longitudinal acoustic phonons $\bar{c}_S^{LA}$, i.e., the speed of sound. We find that the DFT data is in excellent agreement with the Vinet EOS [39] fitted to experimental data up to 40 GPa from Ref. [38], as shown in Fig. 2(c). Further, our calculations agree with room-temperature Brillouin scattering measurements of the speed of sound [40], with the error ranging from 3% to 10%, as shown in Fig. 2(d) in the main text.

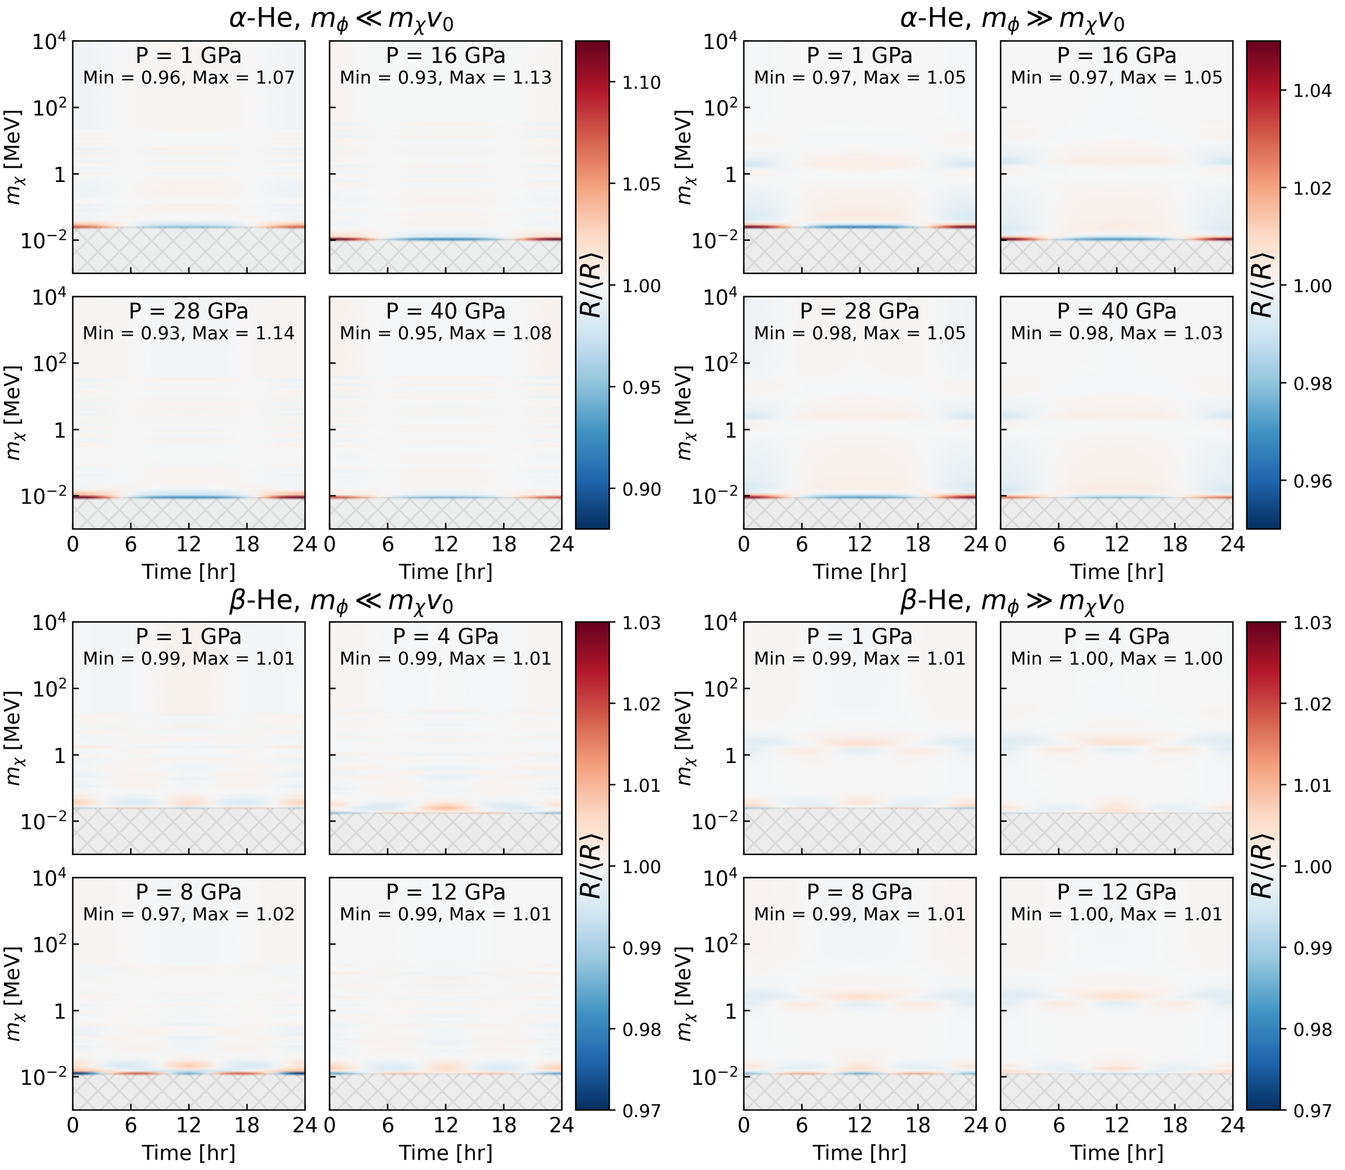


FIG. S2: The variation of the detection rate in $\alpha$- and $\beta$-helium over the course of a day, assuming light ($m_\phi \ll m_\chi v_0$) and heavy ($m_\phi \gg m_\chi v_0$) mediators. The data is shown at four different representative pressures for each phase. The color map corresponds to the rate $R$, normalized by the average daily rate $\langle R \rangle$. The shaded region, corresponding to DM masses where acoustic phonons have no reach, is excluded from our analysis.

* SGriffin@lbl.gov


[1] P. Giannozzi, S. Baroni, N. Bonini, M. Calandra, R. Car, C. Cavazzoni, D. Ceresoli, G. L. Chiarotti, M. Cococcioni, I. Dabo, A. Dal Corso, S. de Gironcoli, S. Fabris, G. Fratesi, R. Gebauer, U. Gerstmann, C. Gougoussis, A. Kokalj, M. Lazzeri, L. Martin-Samos, N. Marzari, F. Mauri, R. Mazzarello, S. Paolini, A. Pasquarello, L. Paulatto, C. Sbraccia, S. Scandolo, G. Sclauzero, A. P. Seitsonen, A. Smogunov, P. Umari, and R. M. Wentzcovitch, Journal of Physics: Condensed Matter **21**, 395502 (2009).

[2] P. Giannozzi, O. Baseggio, P. Bonfà, D. Brunato, R. Car, I. Carnimeo, C. Cavazzoni, S. de Gironcoli, P. Delugas, F. Ferrari Ruffino, A. Ferretti, N. Marzari, I. Timrov, A. Urru, and S. Baroni, The Journal of Chemical Physics **152**, 154105 (2020).

[3] P. E. Blöchl, Physical Review B **50**, 17953 (1994).

[4] A. Dal Corso, Computational Materials Science **95**, 337 (2014).

[5] J. P. Perdew, K. Burke, and M. Ernzerhof, Phys. Rev. Lett. **77**, 3865 (1996).

[6] S. Grimme, J. Antony, S. Ehrlich, and H. Krieg, The Journal of Chemical Physics **132**, 154104 (2010).

[7] D. G. A. Smith, L. A. Burns, K. Patkowski, and C. D. Sherrill, J. Phys. Chem. Lett. **7**, 2197 (2016).

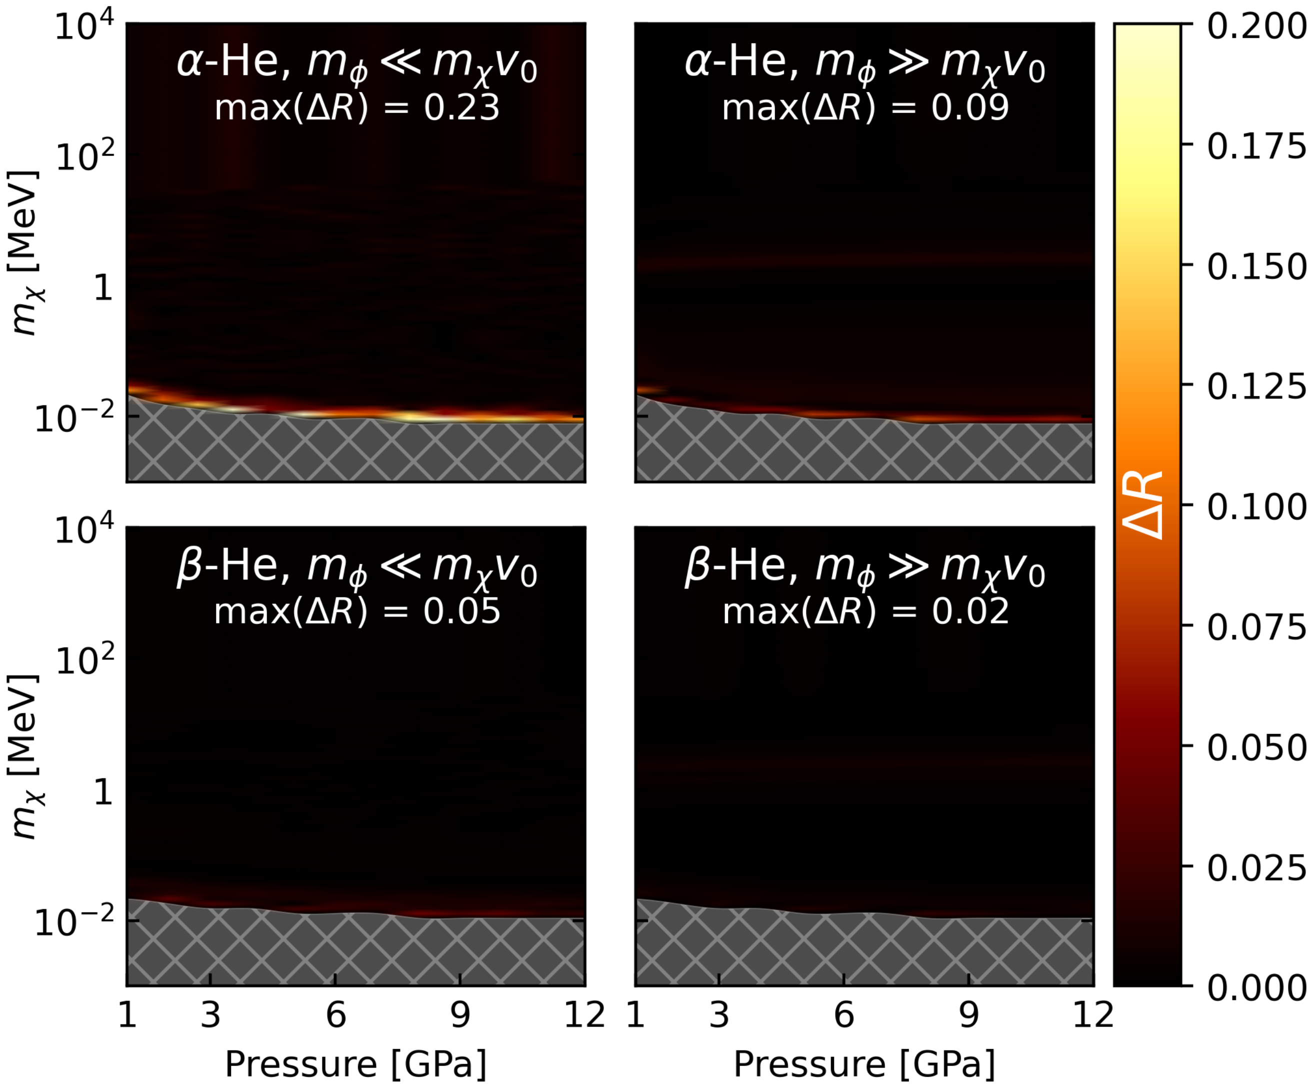


FIG. S3: (a) The total variation in the detection rate $\Delta R$ (Eq. S5) in $\alpha$- and $\beta$-helium for light ($m_\phi \ll m_\chi v_0$) and heavy ($m_\phi \gg m_\chi v_0$) mediators. The data is plotted as a function of pressure and DM mass $m_\chi$. The shaded region corresponds to DM masses where acoustic phonons have no reach, and is excluded from our analysis.


[8] G. Kresse and J. Furthmüller, Computational Materials Science **6**, 15 (1996).
[9] G. Kresse and J. Furthmüller, Phys. Rev. B **54**, 11169 (1996).
[10] G. Kresse and J. Hafner, Phys. Rev. B **47**, 558 (1993).
[11] G. Kresse and J. Hafner, Phys. Rev. B **49**, 14251 (1994).
[12] G. Kresse and D. Joubert, Phys. Rev. B **59**, 1758 (1999).
[13] A. Togo and I. Tanaka, Scripta Materialia **108**, 1 (2015).
[14] O. A. Ashour and S. M. Griffin, DarkMAGIC v0.0.4 (2024).
[15] T. Trickle, Z. Zhang, K. M. Zurek, K. Inzani, and S. M. Griffin, Journal of High Energy Physics **2020**, 36 (2020).
[16] T. Trickle, Z. Zhang, and K. M. Zurek, Physical Review D **105**, 015001 (2022).
[17] S. M. Griffin, K. Inzani, T. Trickle, Z. Zhang, and K. M. Zurek, Physical Review D **101**, 055004 (2020).
[18] R. H. Helm, Physical Review **104**, 1466 (1956).
[19] S. Knapen, T. Lin, and K. M. Zurek, Physical Review D **96**, 115021 (2017).
[20] S. Griffin, S. Knapen, T. Lin, and K. M. Zurek, Physical Review D **98**, 115034 (2018).
[21] J. Eckert, W. Thomlinson, and G. Shirane, Phys. Rev. B **18**, 3074 (1978).
[22] C. Stassis, G. Kline, W. Kamitakahara, and S. K. Sinha, Phys. Rev. B **17**, 1130 (1978).
[23] W. Thomlinson, J. Eckert, and G. Shirane, Phys. Rev. B **18**, 1120 (1978).
[24] M. Dion, H. Rydberg, E. Schröder, D. C. Langreth, and B. I. Lundqvist, Phys. Rev. Lett. **92**, 246401 (2004).
[25] J. P. Perdew, A. Ruzsinszky, G. I. Csonka, O. A. Vydrov, G. E. Scuseria, L. A. Constantin, X. Zhou, and K. Burke, Phys. Rev. Lett. **100**, 136406 (2008).
[26] S. Grimme, S. Ehrlich, and L. Goerigk, Journal of Computational Chemistry **32**, 1456 (2011).

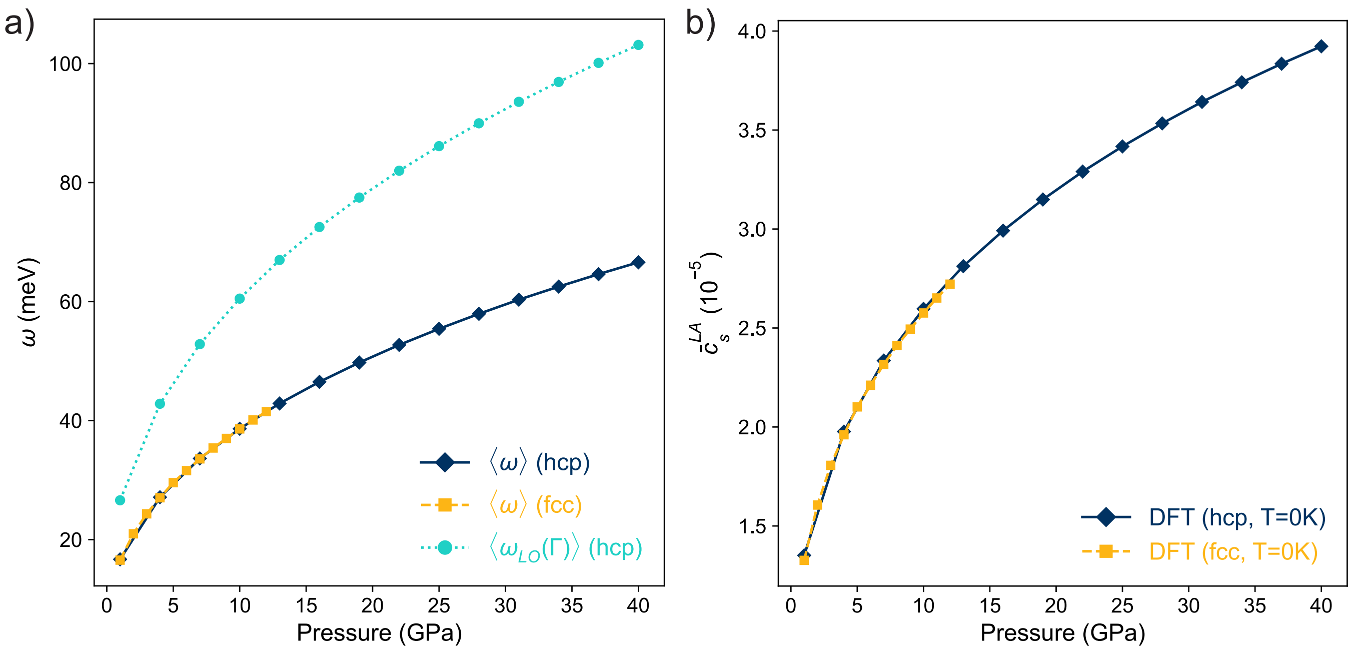


FIG. S4: (a) The phonon frequencies averaged across the entire Brillouin zone, $\langle\omega\rangle$, and the average longitudinal optical phonon frequency near the $\Gamma$ point, $\langle\omega_{\mathrm{LO}}(\Gamma)\rangle$, as a function of pressure. (b) The average speed of sound, $\bar{c}_S^{LA}$ (in natural units where $c = 1$), also as a function of pressure.


[27] A. Ambrosetti, A. M. Reilly, R. A. DiStasio, Jr., and A. Tkatchenko, The Journal of Chemical Physics **140**, 18A508 (2014).
[28] A. Tkatchenko and M. Scheffler, Phys. Rev. Lett. **102**, 073005 (2009).
[29] A. V. Krukau, O. A. Vydrov, A. F. Izmaylov, and G. E. Scuseria, The Journal of Chemical Physics **125**, 224106 (2006).
[30] L. Schimka, J. Harl, and G. Kresse, The Journal of Chemical Physics **134**, 024116 (2011).
[31] J. Klimeš, D. R. Bowler, and A. Michaelides, Phys. Rev. B **83**, 195131 (2011).
[32] K. Berland, D. Chakraborty, and T. Thonhauser, Phys. Rev. B **99**, 195418 (2019).
[33] K. Berland and P. Hyldgaard, Phys. Rev. B **89**, 035412 (2014).
[34] D. Chakraborty, K. Berland, and T. Thonhauser, J. Chem. Theory Comput. **16**, 5893 (2020).
[35] R. Sabatini, T. Gorni, and S. de Gironcoli, Phys. Rev. B **87**, 041108 (2013).
[36] J. Sun, A. Ruzsinszky, and J. P. Perdew, Phys. Rev. Lett. **115**, 036402 (2015).
[37] J. W. Furness, A. D. Kaplan, J. Ning, J. P. Perdew, and J. Sun, J. Phys. Chem. Lett. **11**, 8208 (2020).
[38] P. Loubeyre, R. LeToullec, J. P. Pinceaux, H. K. Mao, J. Hu, and R. J. Hemley, Phys. Rev. Lett. **71**, 2272 (1993).
[39] P. Vinet, J. R. Smith, J. Ferrante, and J. H. Rose, Phys. Rev. B **35**, 1945 (1987).
[40] C.-S. Zha, H.-k. Mao, and R. J. Hemley, Phys. Rev. B **70**, 174107 (2004).


* SGriffin@lbl.gov

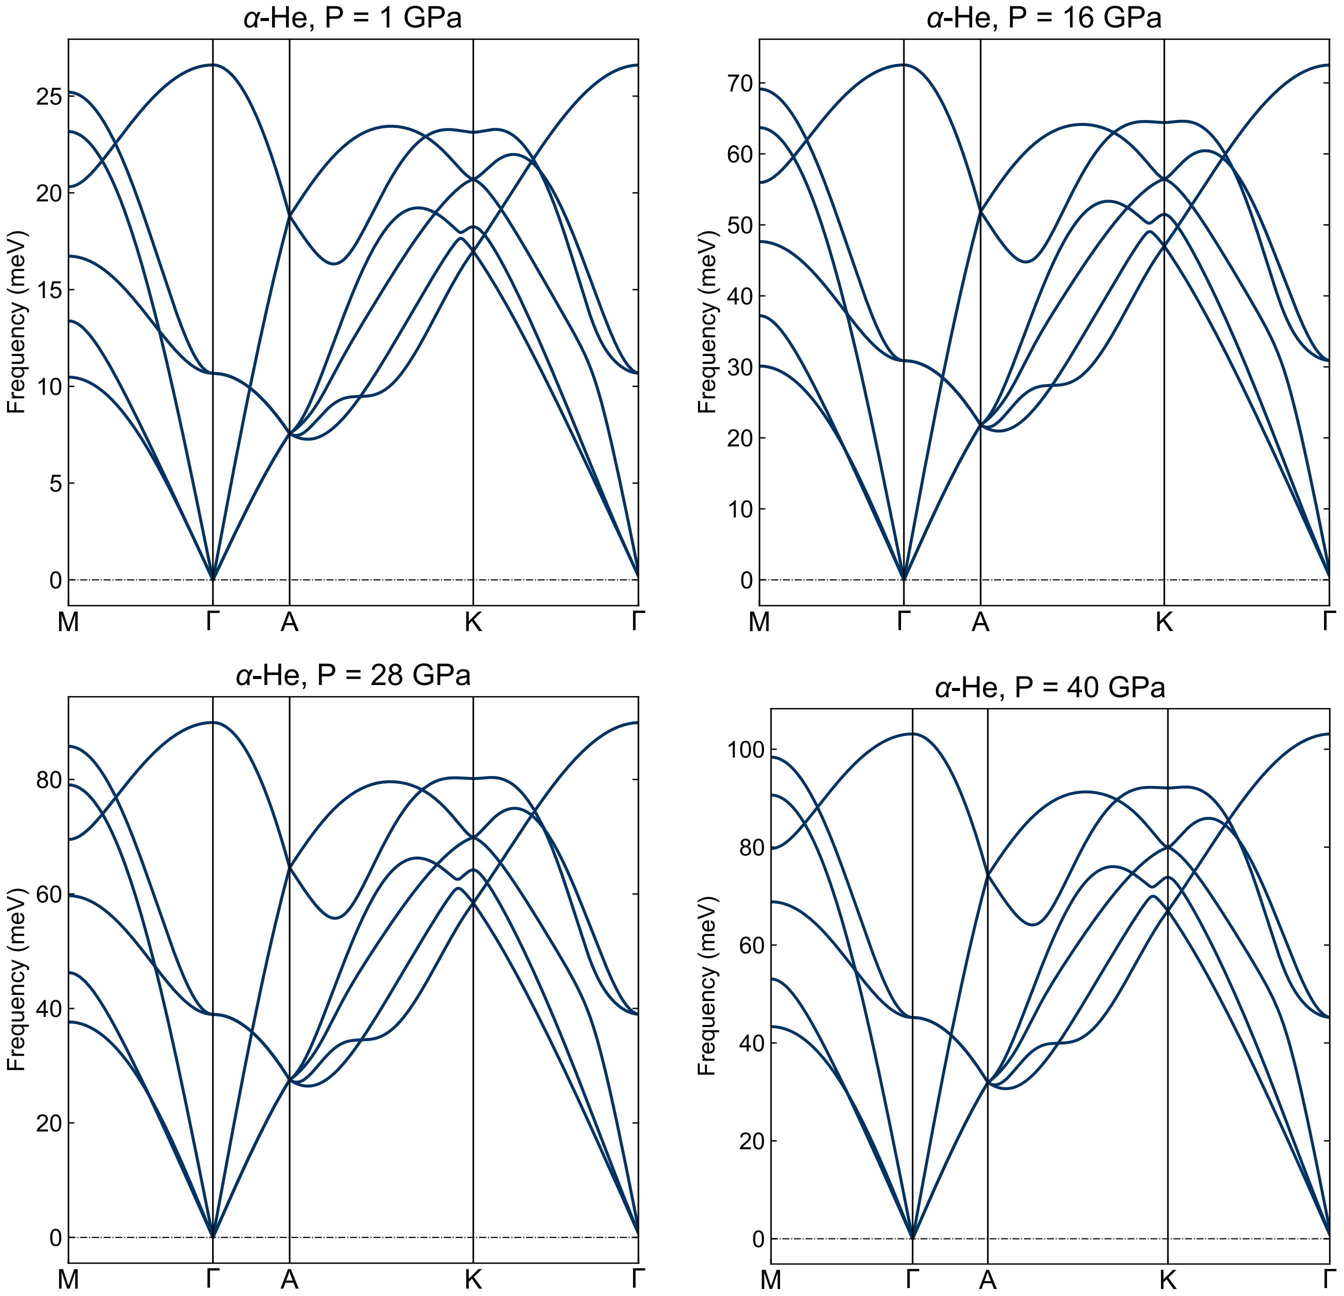


FIG. S5: Phonon band structures of $\alpha$-helium at several representative pressures.

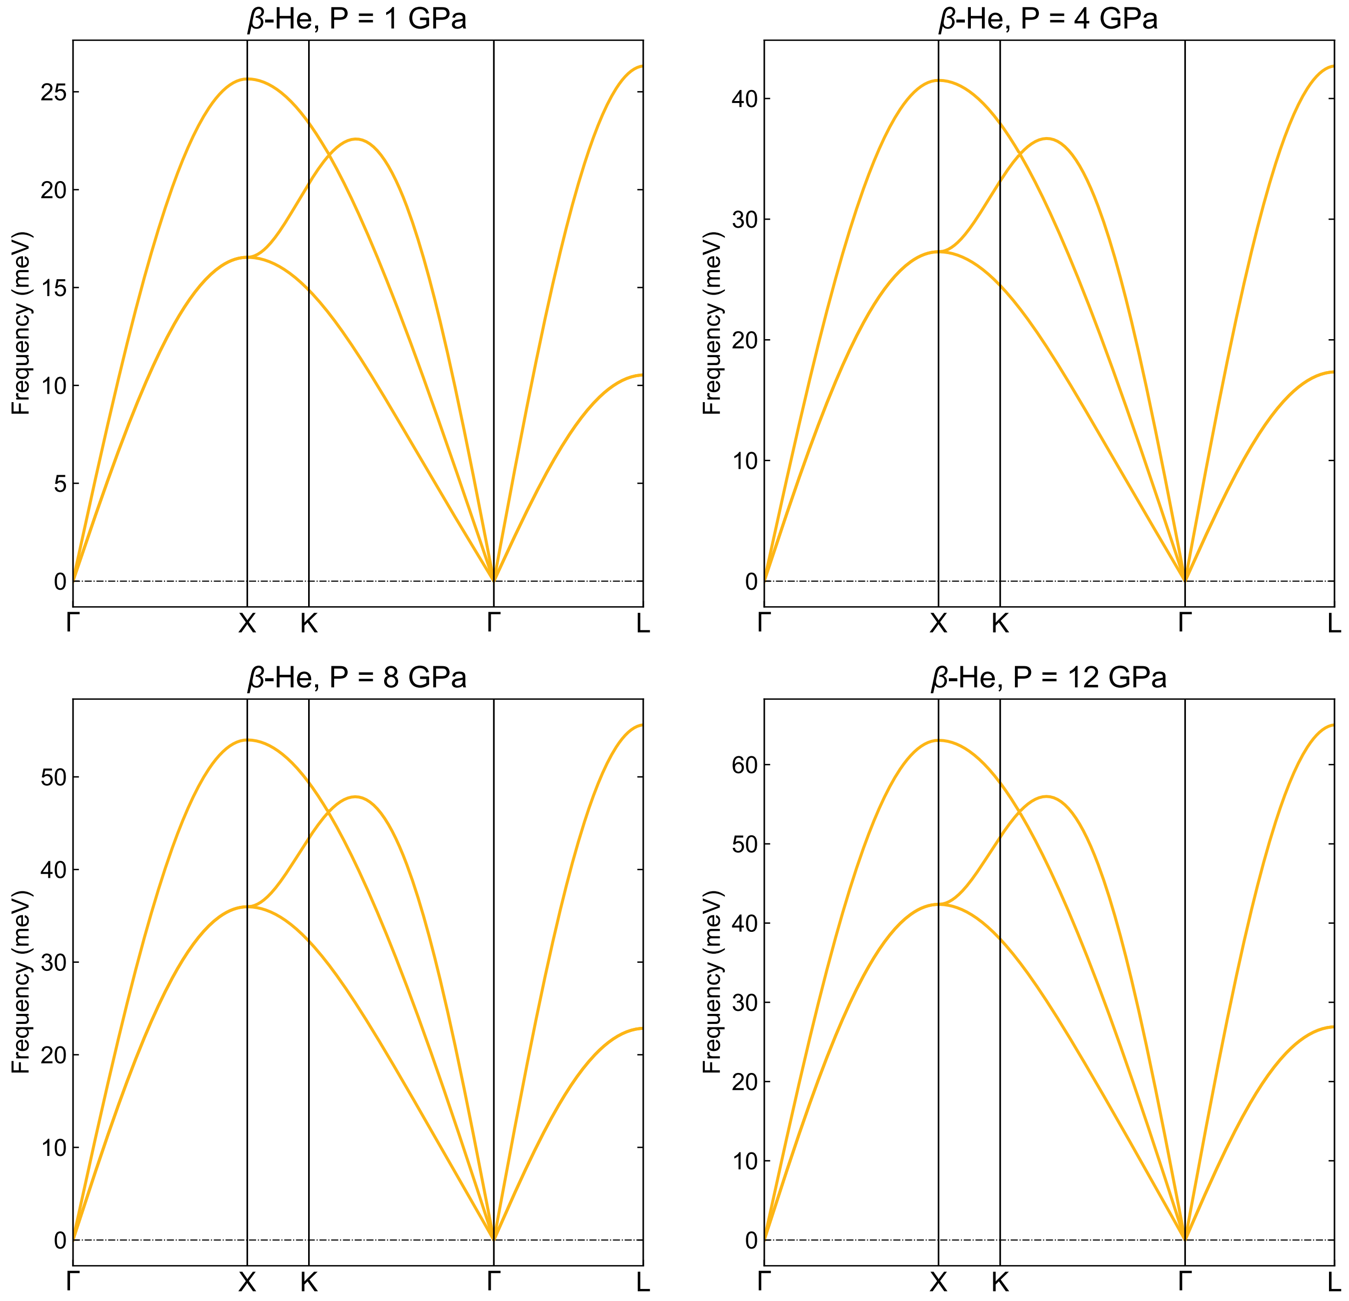


FIG. S6: Phonon band structures of $\beta$-helium at several representative pressures.

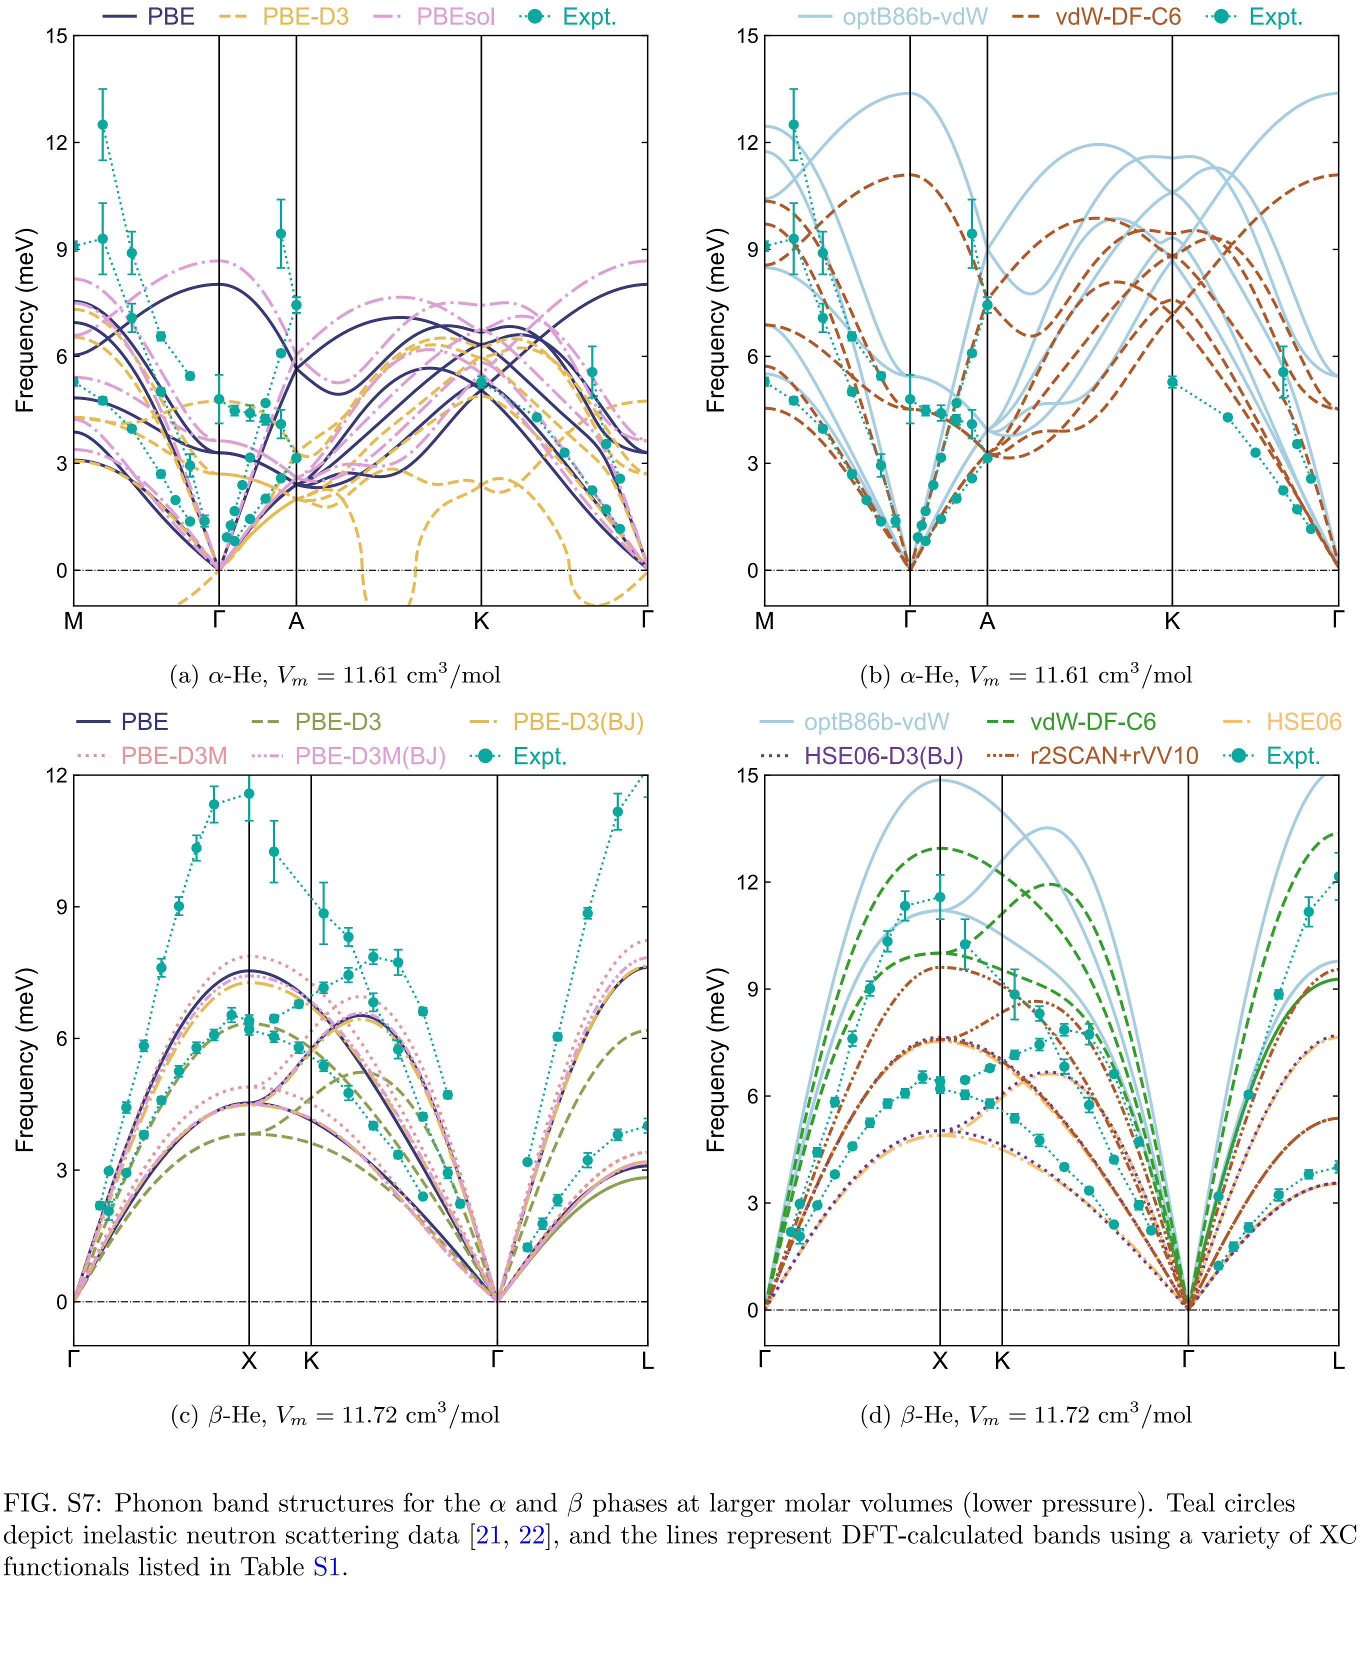


(a) $\alpha$-He, $V_m = 11.61$ cm$^3$/mol

(b) $\alpha$-He, $V_m = 11.61$ cm$^3$/mol

(c) $\beta$-He, $V_m = 11.72$ cm$^3$/mol

(d) $\beta$-He, $V_m = 11.72$ cm$^3$/mol

FIG. S7: Phonon band structures for the $\alpha$ and $\beta$ phases at larger molar volumes (lower pressure). Teal circles depict inelastic neutron scattering data [21, 22], and the lines represent DFT-calculated bands using a variety of XC functionals listed in Table S1.

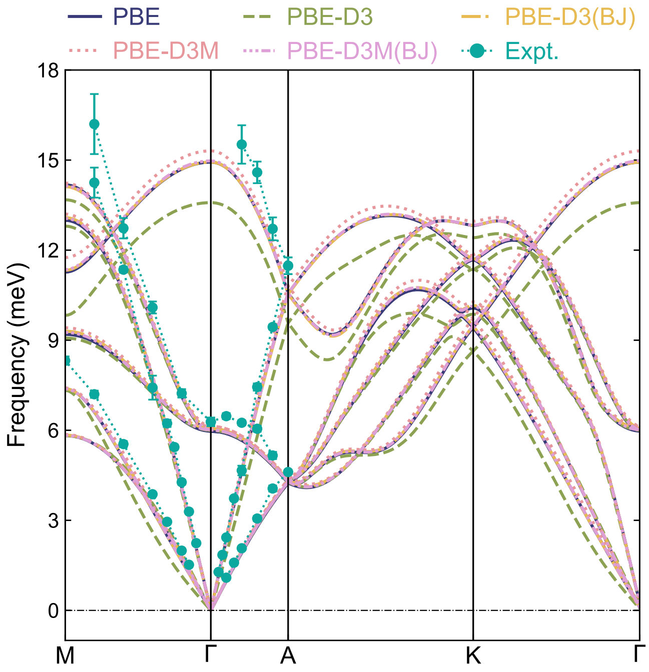


(a) $\alpha$-He, $V_m = 9.41$ cm$^3$/mol

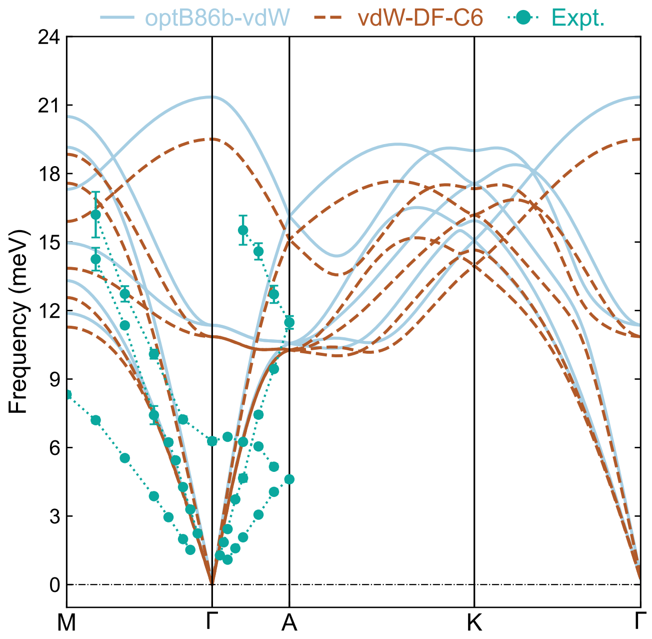


(b) $\alpha$-He, $V_m = 9.41$ cm$^3$/mol

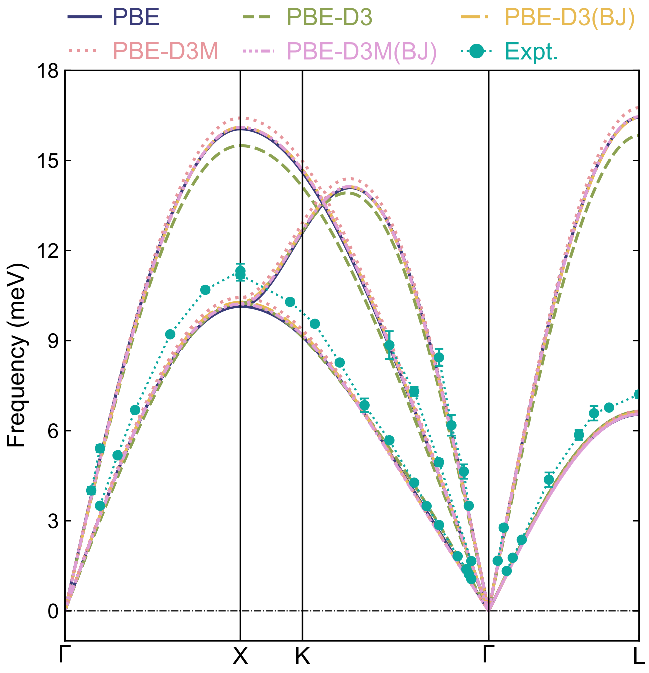


(c) $\beta$-He, $V_m = 9.03$ cm$^3$/mol

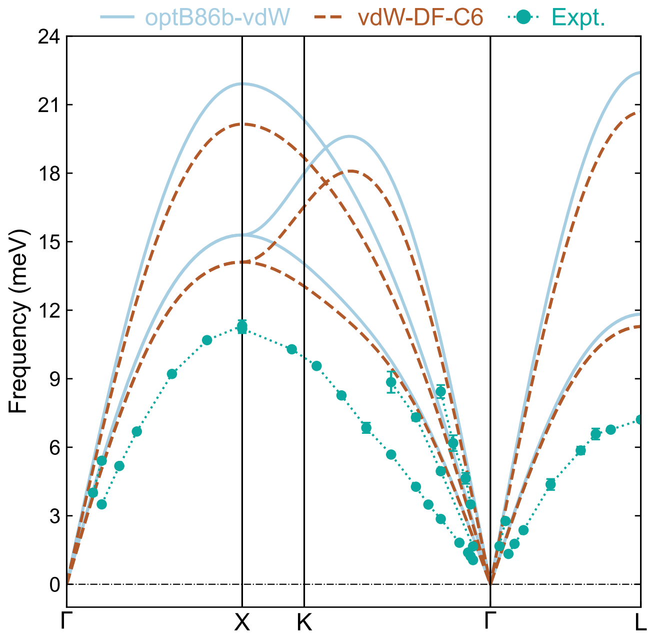


(d) $\beta$-He, $V_m = 9.03$ cm$^3$/mol

FIG. S8: Phonon band structures for the $\alpha$ and $\beta$ phases at smaller molar volumes (higher pressure). Teal circles depict inelastic neutron scattering data [21, 22], and the lines represent DFT-calculated bands using a variety of XC functionals listed in Table S1.

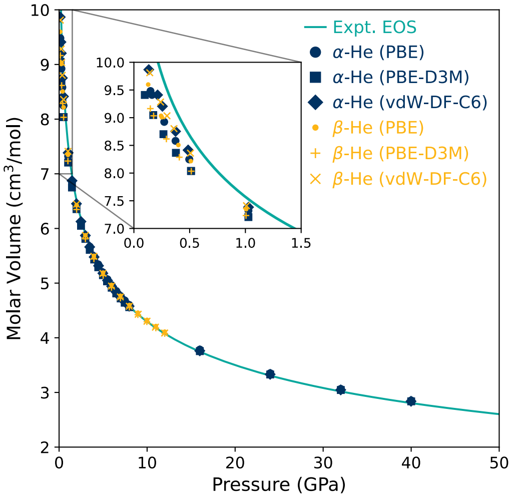


FIG. S9: Comparison of different exchange-correlation functionals' performance in modeling the equation of state of solid helium [38]. Experimental data are sourced from Refs. [21–23].
